# Supplementary material for: Accurate and efficient structure factors in ultrasoft pseudopotential and projector augmented wave DFT
Source: arXiv:2209.12227 source file (2022-09-25)
Supplement: Supplementary file 1 [file supplemental.pdf]

# Supplementary material for
# "Accurate and efficient structure factors in ultrasoft pseudopotential and projector augmented wave DFT"

Benjamin X. Shi,[1,*] Rebecca J. Nicholls,[1] and Jonathan R. Yates[1]

[1] *Department of Materials, University of Oxford, Parks Road, Oxford, OX1 3PH, United Kingdom*

(Dated: September 21, 2022)

## I. EVALUATION OF EFFICIENCY

With our proposed approach in the main text, all of the rapidly varying contributions to the total AE ED no longer need to be placed on the FFT grid, and are instead treated on radial support grids. Thus, the FFT grid, where only the smooth PS valence ED is evaluated, can be kept to its default size. In Fig. S1, we plot the convergence of the $F(111)$ structure factor of Si against the grid size (given in points per Angstrom, ppÅ, along a lattice vector). Superimposed in the same figure, we also plot the (relative) computational resources for the calculations as the FFT grid size increases. The value of $F(111)$ only converges (to 0.001 e) at $\sim$200 ppÅ, which is more than an order of magnitude larger than the default size used (16 ppÅ). For a grid size of $N$ ppÅ, the time and peak RAM required for the calculations scale closely to $\sim \mathcal{O}(N^3)$. This cubic scaling arises because the total number of grid points scales as $N^3$ and it quickly rises to become the dominant contribution to the memory requirements. Similarly, the evaluation of quantities that depend on the fine grid, such as the density as well as exchange-correlation potential, become the dominant factor in the calculations, hence the cubic scaling of the calculation time as well. This cubic scaling of the calculation shows that a converged SF using prior methods would require a three order increase in RAM and time compared to the default grid size, which our methods enable.

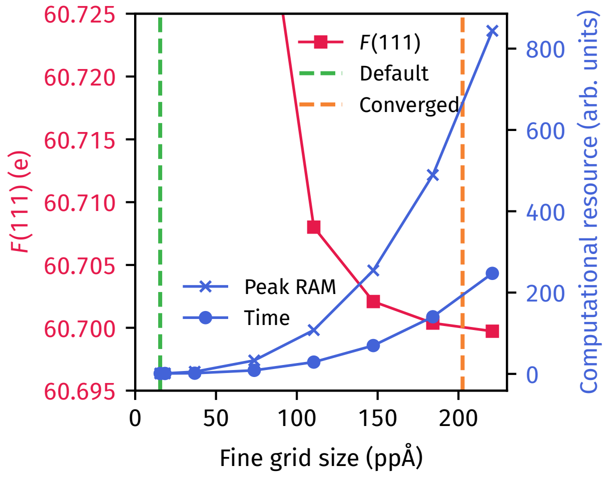


Figure S1. Convergence with fine grid size (given in points per Å, ppÅ, along a lattice vector) of the $F(111)$ structure factor of Si. The calculations were performed on a single core and we plot the time and peak RAM required to complete the calculations in units relative to the default grid size. Calculations were all performed in VASP [1, 2].

* mail@benjaminshi.com

## II. COMPARISON OF STRUCTURE FACTORS FOR LDA AND PBE DENSITY FUNCTIONAL APPROXIMATIONS

In CASTEP, the pseudization scheme for generating on-the-fly pseudopotentials for LDA, GGA and meta-GGA are consistent. As seen in Fig. S2, the difference in the computed structure factors (SFs) between both norm-conserving (NCP) and ultrasoft (USP) pseudopotentials w.r.t. the all-electron (AE) DFT reference follow the same trend for both LDA and PBE (GGA) exchange-correlation functionals.

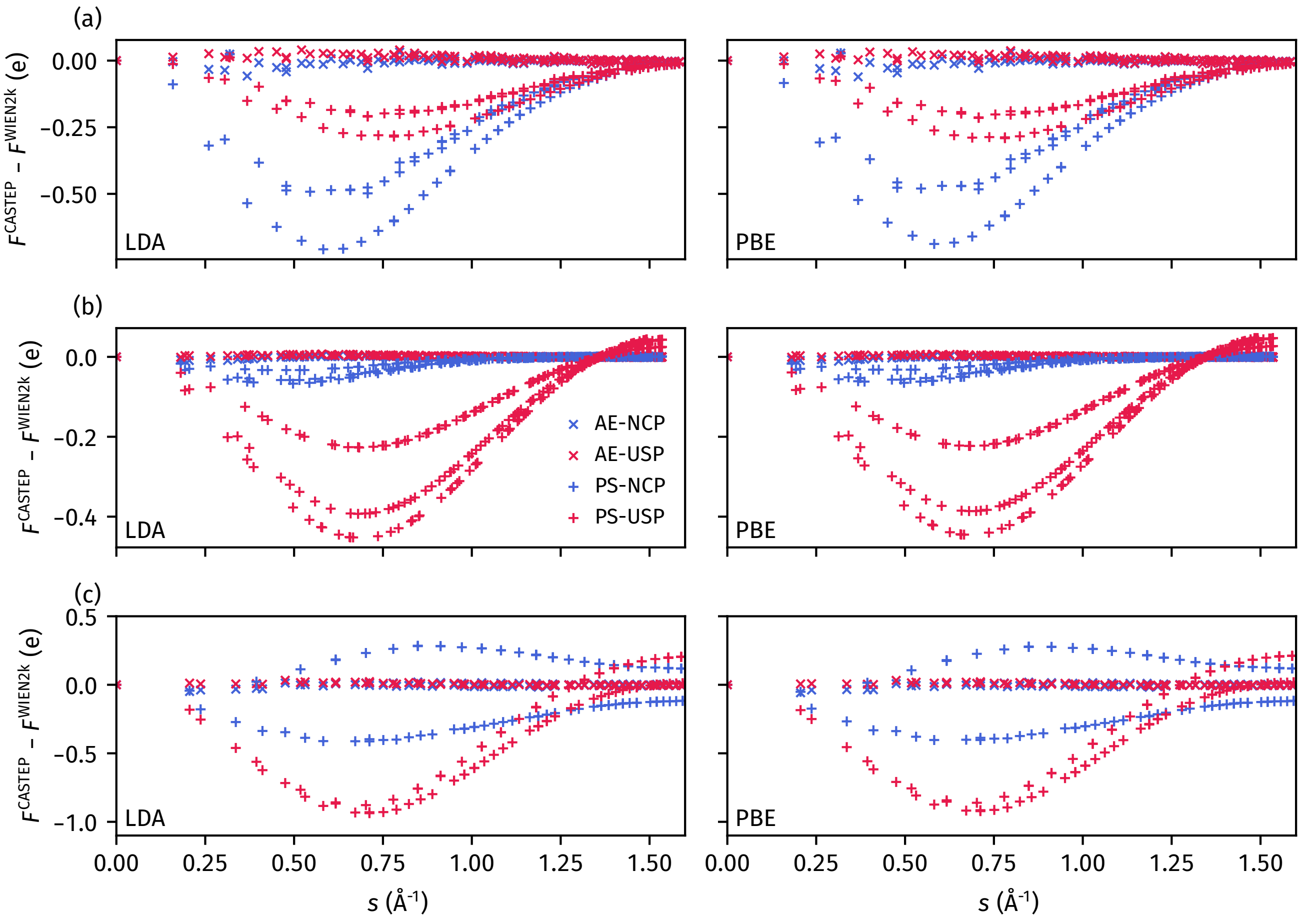


Figure S2. The difference between WIEN2k SF calculations and those obtained from CASTEP as a function of scattering vector $s$ for (a) Si, (b) Mg and (c) MgO for both the LDA (left) and PBE (right) functionals. In CASTEP, PAW DFT calculations were performed employing both USPs and NCPs, with each either using an all-electron (AE) or pseudized (PS) augmentation charge.

## III. COMPUTATIONAL DETAILS AND PSEUDOPOTENTIALS

All input files from the main text and the SI are available in GitHub: benshi97/Data_XRD_Structure_Factor. CASTEP calculations were all performed with a 900 eV energy cutoff and using Monkhorst-Pack $k$-point grids with a 0.014 Å$^{-1}$ spacing to sample the Brillouin zone. This study used on-the-fly generated (OTFG) pseudopotentials for both the NCPs and USPs. The default `C19` set of pseudopotentials were used for the USPs but we found that the default `NCP19` set of NCPs would reproduce the SFs poorly, producing large $R^{\text{WIEN2k}}$ values. These default pseudopotentials did not have projectors which cover the $(l, m)$ angular momentums of all of the valence electrons, so that the basis set used to describe the augmentation charge is not sufficiently complete, resulting in a poor reproduction of the AE ED using the AE augmentation charge. When the NCP pseudopotential set was changed (`SOC19`) to include all chemically relevant angular momenta, we get the high accuracies observed in Table 1 of the

main text. The NCP pseudopotentials for the O atom was further modified with a custom OTFG string (i.e. settings) `2|1.2|23|26|31|20N:21N(qc=9)` for better performance.

WIEN2k calculations were performed with converged settings of $R_{\mathrm{MT}}K_{\mathrm{max}} = 8$ for Mg and Si, and $R_{\mathrm{MT}}K_{\mathrm{max}} = 9$ for MgO, all with $k$-point grid sampling of $< 0.021$ Å$^{-1}$.

## IV. HIRSHFELD PARTITIONING SCHEME FOR APPLYING THE DEBYE-WALLER FACTOR TO STATIC DFT STRUCTURE FACTORS

To match experiments, the effects of thermal vibrations must be incorporated into the static SFs obtained from DFT. Within the independent atom model, the simplest approach to approximate these effects is to multiply each atomic scattering factor by an isotropic temperature factor (see Eqs. 27 and 28 in the main paper), termed the Debye-Waller factor. Within the Vanderbilt ultrasoft pseudopotential and projector augmented wave (PAW) methods, the core electrons and valence augmentation charge can be assigned to specific atomic species, so the same concept for thermal vibrations may be applied to these contributions. However, the pseudized (PS) valence ED does not take up such a representation and there is difficulty in deciding what Debye-Waller factor to use for the PS valence ED in systems with more than one atom type. A similar problem exists in APW+lo AE DFT as well for the interstitial regions in between the muffin-tins and it was dealt with by applying a DW factor that is the average of the atom types. In general, the interstitial region makes up a smaller contribution to the total ED compared to the PS valence ED in PAW DFT (Table S1), so it may be less accurate to apply an average DW factor to the PS valence ED.

Table S1. The separate contributions to the total ED (in brackets) for the Si, Mg and MgO in APW+lo AE DFT WIEN2k and PAW DFT CASTEP calculations. For AE DFT, the ED is separated into (M)uffin-tins and the (I)nterstitial region, while in PAW DFT, the ED is separated into (C)ore, (V)alence and (A)ugmentation contributions, where the last term is 0 in NCPs.

| | AE | | USP | | | NCP | |
|---|---|---|---|---|---|---|---|
| | M | I | C | V | A | C | V |
| Si (112) | 98.68 | 13.32 | 80.00 | 32.35 | -0.35 | 80.00 | 32.00 |
| Mg (24) | 21.56 | 2.44 | 4.00 | 7.41 | 12.59 | 20.00 | 4.00 |
| MgO (80) | 74.56 | 5.44 | 16.00 | 37.67 | 26.33 | 48.00 | 32.00 |

Within CASTEP, we have tried to overcome this potential issue by partitioning the valence ED to specific atoms using the method of Hirshfeld partitioning. It partitions the unit cell pseudo-valence electron density into atomic contributions by defining a weight function $w^j(\mathbf{r})$ for each atom $j$ within the unit cell, which will follow the relationship:

$$\sum_j w^j(\mathbf{r}) = 1 \tag{S1}$$

at any $\mathbf{r}$. The weight functions themselves are derived by finding the relative ratio of the isolated atomic valence electron density $\rho^j_{\mathrm{val}}$ from the atom in each unit cell to the total IAM valence charge density:

$$w^j(\mathbf{r}) = \frac{\sum_{\mathbf{R}} \rho^j_{\mathrm{val}}(\mathbf{r} + \mathbf{r}_j + \mathbf{R})}{\sum_{\mathbf{R}k} \rho^k_{\mathrm{val}}(\mathbf{r} + \mathbf{r}_k + \mathbf{R})}. \tag{S2}$$

The valence electron density for each atom $j$ is assigned according to the equation:

$$\tilde{n}^j_{\mathrm{val}}(\mathbf{r}) = \tilde{n}_{\mathrm{val}} w^j(\mathbf{r}), \tag{S3}$$

which can then be turned into an 'effective' atomic scattering factor to apply individual Debye-Waller factors.

As seen in Table S2, the application of this Hirshfeld partitioning scheme improves over the average DW method for the $R^{\mathrm{EXP}}$ values for MgO.

Table S2. $R^{\mathrm{EXP}}$ (%) values for the Hirshfeld partitioning and average methods of incorporating the Debye-Waller (e.g. temperature) factor into static structure factors. Calculations were performed for the PBE functional in MgO.

| Method | Hirshfeld | Average |
|---|---|---|
| $R^{\mathrm{EXP}}$-factor | 0.297 | 0.335 |

## V. EXPERIMENTAL STRUCTURE FACTORS COMPARED TO PAW DFT AND AE DFT IN SI, MG AND MGO SYSTEMS

Fig. S3 plots the difference between experiment and DFT computed SFs. To be consistent with literature, scattering factors (Eq. 29 in the main paper) were compared for Si. For all three systems, PBE and LDA follow similar trends as a function of scattering vector, probably because both are semilocal functionals that suffer from self-interaction error. In general, the error in PBE w.r.t. experiment is smaller than LDA at most observed scattering vectors.

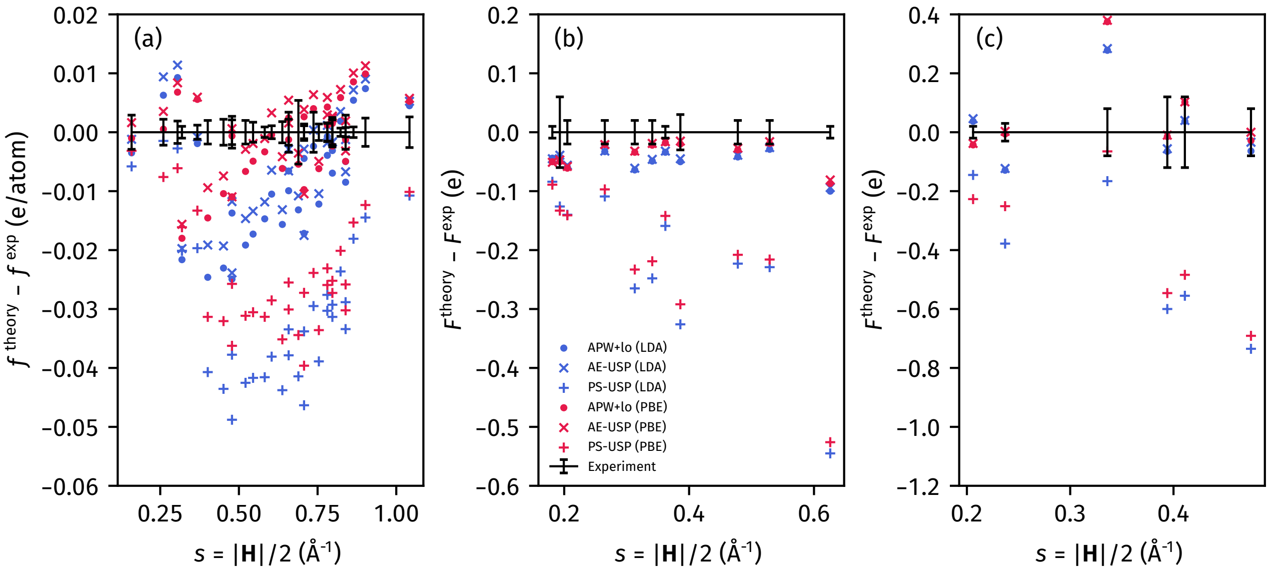


Figure S3. The difference between experimental SFs and those obtained from PAW DFT CASTEP and APW+lo AE DFT WIEN2k as a function of scattering vector $s$ for (a) Si, (b) Mg and (c) MgO.

## VI. CORE AND VALENCE CONTRIBUTIONS TO THE TOTAL SCATTERING FACTOR IN SI

Fig. S4 plots the core and valence (PS valence and augmentation) charge contributions to the total scattering factor of Si. The valence charge contributes significantly to the total structure factor up to $s = 0.2$ Å$^{-1}$ before dropping quickly to give negligible contribution.

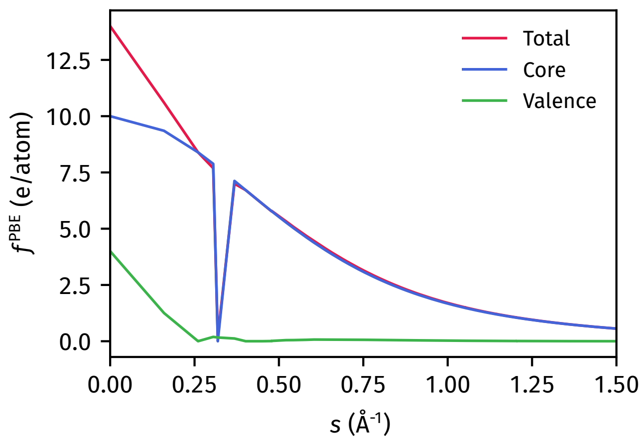


Figure S4. The total, core and valence scattering factors as a function of scattering vector $s$ for Si for the AE-USP PAW DFT method in CASTEP with the PBE functional.

[1] G. Kresse and J. Furthmüller, Efficiency of ab-initio total energy calculations for metals and semiconductors using a plane-wave basis set, Comput. Mater. Sci. **6**, 15 (1996).

[2] G. Kresse and J. Furthmüller, Efficient iterative schemes for ab initio total-energy calculations using a plane-wave basis set, Phys. Rev. B **54**, 11169 (1996).
